# Supplementary material for: Believe Your Model: Distribution-Guided Confidence Calibration
Source: arXiv:2603.03872 source file (2026-03-04)
Supplement: Supplementary file 1 [file case_study.tex]

\clearpage
\newpage
\section{Case Study}
